# Supplementary material for: A note on Horvitz-Thompson estimators for rare subgroup analysis in the presence of interference
Source: arXiv:2001.02719 ancillary file (2020-01-08)
Supplement: Supplementary file 1 [file Supplementary_Materials.pdf]

# Supplementary Materials for: A note on Horvitz-Thompson estimators for rare subgroup analysis in the presence of interference

Erin E Gabriel

January 8, 2020

## 1 Proofs

### Proof of Results

1. Proof of result 1

$$
\begin{aligned}
E\left\{\widehat{\overline{Y}}_j(1;\alpha \mid b) \mid Q_j = 1\right\} &= E\left\{\frac{1}{\sum_i \mathbb{I}_{[w_{ij}\in b]}} \sum_i^{n_j} \frac{Y_{ij} Z_{ij} \mathbb{I}_{[w_{ij}\in b]}}{Pr_\alpha(Z_{ij} = z)} \mid Q_j = 1\right\} \\
&= E\left\{\frac{1}{\sum_i \mathbb{I}_{[w_{ij}\in b]}} \sum_i^{n_j} \frac{Y_{ij} \mathbb{I}_{Z_{ij}=1} \mathbb{I}_{[w_{ij}\in b]}}{Pr_\alpha(Z_{ij} = z)} \mid Q_j = 1\right\} \\
&= \frac{1}{M_{j,b}} \sum_{i=1}^{n_j} \sum_{\nu \in R_\alpha^{n-1}} \frac{Y_{ij} P_\alpha(\mathbf{Z}_{j(i)} = \nu \mid Z_{ij} = z) Pr_\alpha(Z_{ij} = z) \mathbb{I}_{[w_{ij}\in b]}}{Pr_\alpha(Z_{ij} = z)} \\
&= \frac{1}{M_{j,b}} \sum_{i=1}^{n_j} \sum_{\nu \in R_\alpha^{n-1}} Y_{ij} P_\alpha(\mathbf{Z}_{j(i)} = \nu \mid Z_{ij} = z) \mathbb{I}_{[w_{ij}\in b]} \\
&= \frac{1}{M_{j,b}} \sum_{i=1}^{n_j} \overline{Y}_{ij}(1;\alpha) \mathbb{I}_{[w_{ij}\in b]} \\
&= \frac{1}{M_{j,b}} \sum_{i=1}^{n_j} \overline{Y}_{ij}(1;\alpha \mid s) \\
&= \overline{Y}_j(1;\alpha \mid b)
\end{aligned}
$$

$$
\begin{aligned}
E\left\{\widehat{\overline{Y}}_j(\alpha \mid b) \mid Q_j = 1\right\} &= E\left\{\frac{1}{\sum_i \mathbb{I}_{[w_{ij}\in b]}} \sum_i^{n_j} Y_{ij}\mathbb{I}_{[w_{ij}\in b]} \mid Q_j = 1\right\} \\
&= \frac{1}{\sum_i \mathbb{I}_{[w_{ij}\in b]}} \sum_{i=1}^{n_j} \sum_{\nu \in R_\alpha^n} Y_{ij}\Pr_\alpha(\mathbf{Z}_j = \nu)\mathbb{I}_{[w_{ij}\in b]} \\
&= \frac{1}{M_{j,b}} \sum_{i=1}^{n_j} \overline{Y}_{ij}(\alpha)\mathbb{I}_{[w_{ij}\in b]} \\
&= \frac{1}{M_{j,b}} \sum_{i=1}^{n_j} \overline{Y}_{ij}(\alpha \mid b) \\
&= \overline{Y}_j(\alpha \mid b)
\end{aligned}
$$

$$
\mathrm{E}\left\{[\widehat{DE}_j(\alpha \mid b) \mid Q_j = 1]\right\} = DE_j(\alpha \mid b)
$$

Follows directly from result above.

2. Proof of result 2

$$
\begin{aligned}
\mathrm{E}\left\{\widehat{\overline{Y}}(z;\alpha \mid b)\right\} &= \mathrm{E}\left\{\frac{1}{\sum_j \mathbb{I}_{[\sum_i \mathbb{I}_{[w_{ij}\in b]}>0]}} \frac{\sum \widehat{\overline{Y}}_j(z;\alpha \mid b)\mathbb{I}_{[Q_j=1]}}{\Pr_\alpha}\right\} \\
&= \frac{1}{M_b}\mathrm{E}\left\{\frac{\sum \widehat{\overline{Y}}_j(z;\alpha \mid b)\mathbb{I}_{[Q_j=1]}}{\Pr_\alpha}\right\} \\
&= \frac{1}{M_b}\sum \overline{Y}_j(z;\alpha \mid b) \\
&= \overline{Y}(z;\alpha \mid b)
\end{aligned}
$$

$$
\begin{aligned}
\mathrm{E}\left\{\widehat{\widehat{Y}}(\alpha \mid b)\right\} = & \quad \mathrm{E}\left\{\frac{1}{\sum_j \mathbb{I}_{[\sum_i \mathbb{I}_{[w_{ij} \in b]} > 0]}} \frac{\sum \widehat{\widehat{Y}}_j(\alpha \mid b)\mathbb{I}_{[Q_j=1]}}{\mathrm{Pr}_\alpha}\right\} \\
= & \quad \frac{1}{M_b}\mathrm{E}\left\{\frac{\sum \widehat{\widehat{Y}}_j(\alpha \mid b)\mathbb{I}_{[Q_j=1]}}{\mathrm{Pr}_\alpha}\right\} \\
= & \quad \frac{1}{M_b}\sum \overline{Y}_j(\alpha \mid b) \\
= & \quad \overline{Y}(\alpha \mid b)
\end{aligned}
$$

Then the remainder of result 2 follows directly from above.

$\mathrm{E}\left\{\widehat{DE}(\alpha \mid b)\right\} = DE(\alpha \mid b)$ and

$\mathrm{E}\left\{\widehat{OE}(\alpha, \gamma \mid b)\right\} = OE(\alpha, \gamma \mid b)$ and

$\mathrm{E}\left\{\widehat{IE}(\alpha, \gamma \mid b)\right\} = IE(\alpha, \gamma \mid b)$ and

$\mathrm{E}\left\{\widehat{TE}(\alpha, \gamma \mid b)\right\} = TE(\alpha, \gamma \mid b)$

3. Proof of result 3:

Follows directly from Hudgens and Halloran [2008] with only minor alterations. Either a group has $d_j \in B$ or not, if $d_j \in B$, then the proofs follow directly because they are the same estimators as $\Pr(Q_j = 1) = K/J$, and there is no subgroup analysis. If not they are zero, which by our definition of the estimands makes them unbiased.

$$
\begin{aligned}
\mathrm{E}\left\{\widehat{\widehat{Y}}(z; \alpha \mid B)\right\} = & \quad \mathrm{E}\left\{\frac{1}{\sum_{j=1}^J \mathbb{I}_{[d_j \in B]}} \sum_{j=1}^J \frac{\widehat{\widehat{Y}}_j(z; \alpha \mid B)\mathbb{I}_{[Q_j=1]}}{\mathrm{Pr}_\alpha}\right\} \\
= & \quad \frac{1}{M_B}\sum_{j=1}^J \frac{\mathrm{E}\{\widehat{\widehat{Y}}_j(z; \alpha)\}\Pr(Q_j = 1)\mathbb{I}_{[d_j \in B]}}{\mathrm{Pr}_\alpha} \\
= & \quad \frac{1}{M_B}\sum_{j=1}^J \overline{Y}_j(1; \alpha)\mathbb{I}_{[d_j \in B]} \\
= & \quad \overline{Y}(1; \alpha \mid B)
\end{aligned}
$$

and

$$
\begin{aligned}
\mathrm{E}\left\{\widehat{\overline{Y}}(\alpha \mid B)\right\} &= \mathrm{E}\left\{\frac{1}{\sum_{j=1}^{J}\mathbb{I}_{[d_j\in B]}}\sum_{j=1}^{J}\frac{\widehat{\overline{Y}}_j(\alpha \mid B)\mathbb{I}_{[Q_j=1]}}{\Pr_\alpha}\right\} \\
&= \frac{1}{M_B}\sum_{j=1}^{J}\frac{\mathrm{E}\{\widehat{\overline{Y}}_j(\alpha)\}\Pr(Q_j=1)\mathbb{I}_{[d_j\in B]}}{\Pr(Q_j=1)} \\
&= \frac{1}{M_B}\sum_{j=1}^{J}\overline{Y}_j(\alpha)\mathbb{I}_{[d_j\in B]} \\
&= \overline{Y}(\alpha \mid B)
\end{aligned}
$$

Then the remainder of result 3 follows directly from above.

$\mathrm{E}\left\{\widehat{DE}(\alpha \mid B)\right\} = DE(\alpha \mid B)$ and

$\mathrm{E}\left\{\widehat{OE}(\alpha,\gamma \mid B)\right\} = OE(\alpha,\gamma \mid B)$ and

$\mathrm{E}\left\{\widehat{IE}(\alpha,\gamma \mid B)\right\} = IE(\alpha,\gamma \mid B)$ and

$\mathrm{E}\left\{\widehat{TE}(\alpha,\gamma \mid B)\right\} = TE(\alpha,\gamma \mid B)$

4. Proof of result 4

$$
\begin{aligned}
\mathrm{E}\left\{\widehat{\overline{Y}}_j(1;\alpha \mid B,b) \mid Q=1\right\} &= \mathrm{E}\left\{\mathbb{I}_{[d_j\in B]}\frac{1}{\sum_i \mathbb{I}_{[w_{ij}\in b]}}\sum_{i}^{n_j}\frac{Y_{ij}Z_{ij}\mathbb{I}_{[w_{ij}\in b]}}{P_\alpha^j} \mid Q=1\right\} \\
&= \mathbb{I}_{[d_j\in B]}\mathrm{E}\left\{\widehat{\overline{Y}}_j(1;\alpha \mid b) \mid Q=1\right\} \\
&= \mathbb{I}_{[d_j\in B]}\overline{Y}_j(1;\alpha \mid b) \\
&= \overline{Y}_j(1;\alpha \mid B,b)
\end{aligned}
$$

$$
\begin{aligned}
\mathrm{E}\left\{\widehat{\widehat{Y}}_j(\alpha \mid B, b) \mid Q=1\right\} &= \mathrm{E}\left\{\mathbb{I}_{[d_j \in B]} \frac{1}{\sum_i \mathbb{I}_{[w_{ij} \in b]}} \sum_i^{n_j} \frac{Y_{ij}\mathbb{I}_{[w_{ij} \in b]}}{P_\alpha^j} \mid Q=1\right\} \\
&= \mathbb{I}_{[d_j \in B]} \mathrm{E}\left\{\widehat{\widehat{Y}}_j(\alpha \mid b) \mid Q=1\right\} \\
&= \mathbb{I}_{[d_j \in B]} \overline{Y}_j(\alpha \mid b) \\
&= \overline{Y}_j(\alpha \mid B, b)
\end{aligned}
$$

5. Proof of result 5

$$
\begin{aligned}
\mathrm{E}\left\{\widehat{\widehat{Y}}(z; \alpha \mid B, b)\right\} &= \mathrm{E}\left\{\frac{1}{\sum_j \mathbb{I}_{[d_j \in B]}\mathbb{I}_{[\sum w_{ij} \in b]>0}} \frac{\sum \widehat{\widehat{Y}}_j(z; \alpha \mid B, b)\mathbb{I}_{[Q_j=1]}}{\mathrm{Pr}_\alpha}\right\} \\
&= \frac{1}{\sum_j \mathbb{I}_{[d_j \in B]}\mathbb{I}_{[\sum w_{ij} \in b]>0}} \sum \mathrm{E}\left\{\widehat{\widehat{Y}}(z; \alpha \mid B, b)\right\} \\
&= \frac{1}{M_{B,b}} \sum \overline{Y}_j(z; \alpha \mid B, b) \\
&= \overline{Y}(z; \alpha \mid B, b)
\end{aligned}
$$

$$
\begin{aligned}
\mathrm{E}\left\{\widehat{\widehat{Y}}(\alpha \mid B, b)\right\} &= \mathrm{E}\left\{\frac{1}{\sum_j \mathbb{I}_{[d_j \in B]}\mathbb{I}_{[\sum w_{ij} \in b]>0}} \frac{\sum \widehat{\widehat{Y}}_j(\alpha \mid B, b)\mathbb{I}_{[Q_j=1]}}{\mathrm{Pr}_\alpha}\right\} \\
&= \frac{1}{\sum_j \mathbb{I}_{[d_j \in B]}\mathbb{I}_{[\sum w_{ij} \in b]>0}} \sum \mathrm{E}\left\{\widehat{\widehat{Y}}(\alpha \mid B, b)\right\} \\
&= \frac{1}{M_{B,b}} \sum \overline{Y}_j(\alpha \mid B, b) \\
&= \overline{Y}(\alpha \mid B, b)
\end{aligned}
$$

The unbiasedness of the contrast estimators then follows directly:

$\widehat{DE}(\alpha \mid B, b) = \widehat{\widehat{Y}}(1; \alpha \mid B, b) - \widehat{\widehat{Y}}(0; \alpha \mid B, b)$

$\widehat{OE}(\alpha, \gamma \mid B, b) = \widehat{\widehat{Y}}(\alpha \mid B, b) - \widehat{\widehat{Y}}(\gamma \mid B, b)$

$$\widehat{IE}(\alpha, \gamma \mid B, b) = \widehat{\widehat{\overline{Y}}}(0; \alpha \mid B, b) - \widehat{\widehat{\overline{Y}}}(0; \gamma \mid B, b)$$

$$\widehat{TE}(\alpha, \gamma \mid B, b) = \widehat{\widehat{\overline{Y}}}(1; \alpha \mid B, b) - \widehat{\widehat{\overline{Y}}}(0; \gamma \mid B, b)$$

**Theorem 1** $\mid b$

Assuming that all $d_j \in B$, thus we are only conditioning on $w_{ij} \in b$, and then under assumptions a-d and $M_{j,b} > 0$ and $n_j P_\alpha - 1 > 0$

$$\mathrm{E}\{\widehat{\mathrm{Var}}[\widehat{\widehat{\overline{Y}}}_j(z; \alpha \mid b) \mid Q_j = 1] \mid Q_j = 1\} = \mathrm{Var}[\widehat{\widehat{\overline{Y}}}_j(z; \alpha \mid b) \mid Q_j = 1].$$

where

$$\widehat{\mathrm{Var}}[\widehat{\widehat{\overline{Y}}}_j(1; \alpha \mid b) \mid Q_j = 1] \equiv$$
$$\left(1 - P_\alpha^j\right) \frac{\sum_{i=1}^{n_j} Z_{ij} \left[Y_{ij} Z_{ij} \mathbb{I}_{[w_{ij} \in b]}(n_j/M_{j,b}) - \widehat{\widehat{\overline{Y}}}_j(1; \alpha \mid b)\right]^2}{(n_j P_\alpha^j - 1) n_j P_\alpha^j}$$

with $\widehat{\mathrm{Var}}[\widehat{\widehat{\overline{Y}}}_j(0; \alpha \mid b) \mid Q_j = 1]$ as well as $\widehat{\mathrm{Var}}[\widehat{\widehat{\overline{Y}}}_j(1; \gamma \mid b) \mid Q_j = 0]$ defined similarly.

**Proof Theorem 1 is this setting**

Noting that $\overline{Y}_j(1; \alpha \mid b) = \frac{1}{n_j} \sum_i \overline{Y}_{ij}(1; \alpha \mid b)(n/M_{j,b})$. one can write $\mathrm{Var}[\widehat{\widehat{\overline{Y}}}_j(1; \alpha \mid b) \mid Q_j = 1]$ as

$$\left(1 - P_\alpha^j\right) \frac{\sum_{i=1}^{n_j} \left[\overline{Y}_{ij}(1; \alpha \mid b)(n_j/M_{j,b}) - \overline{Y}_j(1; \alpha \mid b)\right]^2}{(n_j - 1) n_j P_\alpha^j}$$

because $\overline{Y}_j(1; \alpha \mid b)$ is the mean of a simple random sample from the $\overline{Y}_{1j}(1; \alpha \mid b)(n/M_{j,b}), \ldots, \overline{Y}_{n_j,j}(1; \alpha \mid b)(n/M_{j,b})$. Noting this this proof, and then those that build on it, follow directly from standard finite population sampling without replacement. I work through the proofs from completeness and clarity.

Let

$$S^2 = \frac{\sum_{i=1}^{n_j} \left[\overline{Y}_{ij}(1; \alpha \mid b)(n_j/M_{j,b}) - \overline{Y}_j(1; \alpha \mid b)\right]^2}{(n_j - 1)}$$

and

$$\sigma^2 = \frac{\sum_{i=1}^{n_j} \left[\overline{Y}_{ij}(1; \alpha \mid b)(n_j/M_{j,b}) - \overline{Y}_j(1; \alpha \mid b)\right]^2}{n_j} = \frac{(n_j - 1)}{n_j} S^2$$

Note that then $E\{\overline{Y}_{ij}(1;\alpha \mid b)(n_j/M_{j,b})^2\} = \sigma^2 + \overline{Y}_j(1;\alpha \mid b)^2$

$$\begin{aligned}
\mathrm{E}\{\widehat{\mathrm{Var}}[\widehat{\overline{Y}}_j(1;\alpha \mid b) \mid Q_j = 1] \mid Q_j = 1\} = & \quad \mathrm{E}\left\{ \left(1 - P_\alpha^j\right) \frac{\sum_{i=1}^{n_j} Z_{ij}\left[Y_{ij} Z_{ij} \mathbb{I}_{[w_{ij} \in b]}(n_j/M_{j,b}) - \widehat{\overline{Y}}_j(1;\alpha \mid b)\right]^2}{(n_j P_\alpha^j - 1) n_j P_\alpha^j} \right\} \\
= & \quad \left(1 - P_\alpha^j\right) \frac{1}{n_j P_\alpha^j} \mathrm{E}\left\{ \frac{\sum_{i=1}^{n_j} Z_{ij}\left[\overline{Y}_{ij}(1;\alpha \mid b)(n_j/M_{j,b}) - \widehat{\overline{Y}}_j(1;\alpha \mid b)\right]^2}{(n_j P_\alpha^j - 1)} \right\} \\
= & \quad \left(1 - P_\alpha^j\right) \frac{1}{n_j P_\alpha^j} \frac{\sum_{i=1}^{n_j}\left[\overline{Y}_{ij}(1;\alpha \mid b)(n_j/M_{j,b}) - \overline{Y}_j(1;\alpha \mid b)\right]^2}{(n_j - 1)}
\end{aligned}$$

because

$$\begin{aligned}
& \mathrm{E}\left\{ \mathrm{E}\left[ \frac{\sum_{i=1}^{n_j} Z_{ij}\left(Y_{ij} Z_{ij} \mathbb{I}_{[w_{ij} \in b]}(n_j/M_{j,b}) - \widehat{\overline{Y}}_j(1;\alpha \mid b)\right)^2}{(n_j P_\alpha^j - 1)} \mid Z_{ij} = 1 \right] \mid Q_j = 1 \right\} \\
& = \frac{1}{n_j P_\alpha^j - 1} \mathrm{E}\{\mathrm{E}[\sum_{i=1}^{n_j} Z_{ij}(Y_{ij} Z_{ij} \mathbb{I}_{[w_{ij} \in b]}(n_j/M_{j,b}))^2 \mid Z_{ij} = 1, Q_j = 1] \\
& -\mathrm{E}[2\sum_{i=1}^{n_j} Z_{ij} Y_{ij} Z_{ij} \mathbb{I}_{[w_{ij} \in b]}(n_j/M_{j,b}) \widehat{\overline{Y}}_j(1;\alpha \mid b) \mid Z_{ij} = 1, Q_j = 1] \\
& +\mathrm{E}[\sum_{i=1}^{n_j} Z_{ij} \widehat{\overline{Y}}_j(1;\alpha \mid b)^2 \mid Z_{ij} = 1, Q_j = 1] Q_j = 1\} \\
& = \frac{1}{n_j P_\alpha^j - 1} \mathrm{E}\{\mathrm{E}[\sum_{i=1}^{n_j} Z_{ij}(\overline{Y}_{ij}(1;\alpha \mid b)(n_j/M_{j,b}))^2 \mid Z_{ij} = 1, Q_j = 1] \\
& -\mathrm{E}[2 Z_{ij} n_j \widehat{\overline{Y}}_j(1;\alpha \mid b)^2 \mid Z_{ij} = 1, Q_j = 1] \\
& +\mathrm{E}[n_j Z_{ij} \widehat{\overline{Y}}_j(1;\alpha \mid b)^2 \mid Z_{ij} = 1, Q_j = 1] \mid Q_j = 1\} \\
= & \frac{1}{n_j P_\alpha^j - 1}\left( n_j P_\alpha^j((n_j - 1)/n_j) S^2 + n_j P_\alpha^j \overline{Y}_j(1;\alpha \mid b)^2 - n_j P_\alpha^j \mathrm{Var}(\widehat{\overline{Y}}_j(1;\alpha \mid b)) - n_j P_\alpha^j \overline{Y}_j(1;\alpha \mid b)^2 \right) \\
& = \frac{1}{n_j P_\alpha^j - 1}\left( n_j P_\alpha^j((n_j - 1)/n_j) S^2 - n_j P_\alpha^j (1 - P_\alpha^j)/(P_\alpha^j n_j) S^2 \right) = S^2
\end{aligned}$$

noting that $\mathrm{E}\{\mathrm{E}[Z_{ij}\widehat{\overline{Y}}_j(1;\alpha \mid b) \mid Z = 1, Q_j = 1] \mid Q_j = 1\} = \mathrm{E}\{Z_{ij}\overline{Y}_j(1;\alpha \mid b)\} = P_\alpha^j \overline{Y}_j(1;\alpha \mid b)$

**Theorem 2** $\mid b$

Assuming that all $d_j \in B$, thus we are only conditioning on $w_{ij} \in b$ and then under assumptions a-d and $M_b > 0$ and $n_j P_\alpha^j - 1 > 0$

$$\mathrm{E}\{\widehat{\mathrm{Var}}[\widehat{\overline{Y}}(z;\alpha \mid b)]\} = \mathrm{Var}[\widehat{\overline{Y}}(z;\alpha \mid b)].$$

where

$$\widehat{\mathrm{Var}}[\widehat{\overline{Y}}(1;\alpha \mid b)] \equiv (1 - Pr_\alpha)\, \frac{\sum_{j=1}^{J} \mathbb{I}_{[Q_j=1]} \left[\widehat{\overline{Y}}_j(z;\alpha \mid b)(J/M_b) - \widehat{\overline{Y}}(z;\alpha \mid B)\right]^2}{(JPr_\alpha - 1)JPr_\alpha}$$
$$+ \frac{1}{Pr_\alpha M_b^2} \sum_{j=1}^{J} g_{M_{j,b}}(\widehat{\mathrm{Var}}[\widehat{Y}_j(z;\alpha \mid b)])\mathbb{I}_{[Q_j=1]}$$

with $\widehat{\mathrm{Var}}[\widehat{\overline{Y}}(z;\gamma \mid b)]$ defined similarly.

**Proof Theorem 2 in this setting**

and

$$S_P^2 = \frac{\sum_{j=1}^{J} \left[\overline{Y}_j(z;\alpha \mid b)(J/M_b) - \overline{Y}(z;\alpha \mid b)\right]^2}{(J-1)}$$

Note that $\widehat{\overline{Y}}(z;\alpha \mid b)$ can be thought of as a the mean of a simple random sample from the $\widehat{\overline{Y}}_1(z;\alpha \mid b)(J/M_b), \ldots, \widehat{\overline{Y}}_J(z;\alpha \mid b)(J/M_b)$,

Based on this one can write

$$\mathrm{Var}[\widehat{\overline{Y}}(z;\alpha \mid b)] = (1 - Pr_\alpha)\frac{S_P^2}{Pr_\alpha J} + \frac{1}{Pr_\alpha M_b^2} \sum_{j \in \mathbb{J}^b} (1 - P_\alpha^j)\frac{S^2}{n_j P_\alpha^j}.$$

$$\widehat{\mathrm{Var}}[\widehat{\overline{Y}}(z;\alpha \mid b)] \equiv (1 - Pr_\alpha)\, \frac{\sum_{j=1}^{J} \mathbb{I}_{[Q_j=1]} \left[\widehat{\overline{Y}}_j(z;\alpha \mid b)(J/M_b) - \widehat{\overline{Y}}(z;\alpha \mid b)\right]^2}{(JPr_\alpha - 1)JPr_\alpha}$$
$$+ \frac{\sum_{j \in \mathbb{J}^b} \widehat{\mathrm{Var}}[\widehat{Y}_j(z;\alpha \mid b)]\mathbb{I}_{[Q_j=1]}}{Pr_\alpha M_b^2}$$

$\mathrm{E}[\widehat{\mathrm{Var}}(\widehat{\widehat{Y}}(z;\alpha \mid b))] = \mathrm{E}[\mathrm{E}[\widehat{\mathrm{Var}}(\widehat{\widehat{Y}}(z;\alpha \mid b)) \mid Q=1]] =$

$$\mathrm{E}\left\{\mathrm{E}\left[(1-Pr_\alpha)\frac{\sum_{j=1}^{J}\mathbb{I}_{[Q_j=1]}\left\{\widehat{\widehat{Y}}_j(z;\alpha \mid b)(J/M_b)-\widehat{\widehat{Y}}(z;\alpha \mid b)\right\}^2}{(JPr_\alpha-1)JPr_\alpha} \mid Q_j=1\right]+\mathrm{E}\left[\frac{\sum_{j\in\mathbb{J}^b}\widehat{\mathrm{Var}}[\widehat{Y}_j(z;\alpha \mid b)]\mathbb{I}_{[Q_j=1]}}{(Pr_\alpha M_b^2)} \mid Q_j=1\right]\right\}$$

$$= (1-Pr_\alpha)\frac{S_P^2}{Pr_\alpha J}+\left[(1-Pr_\alpha)\frac{1}{JPr_\alpha}\frac{J^2}{M_b^2}\frac{1}{J}+\frac{Pr_\alpha}{Pr_\alpha M_b^2}\right]\sum_{j\in\mathbb{J}^b}(1-P_\alpha^j)\frac{S^2}{n_jP_\alpha^j}$$

$$= (1-Pr_\alpha)\frac{S_P^2}{Pr_\alpha J}+\frac{1}{P_\alpha M_b^2}\sum_{j\in\mathbb{J}^b}(1-P_\alpha^j)\frac{S^2}{n_jP_\alpha^j}$$

$$= \mathrm{Var}[\widehat{\widehat{Y}}(z;\alpha \mid b)]$$

**Theorem 1** $\mid B$

Assuming that all $w_{ij} \in b$, thus we are only conditioning on $d_j \in B$, then under assumptions a-d and $n_jP_\alpha^j - 1 > 0$

$$\mathrm{E}\{\widehat{\mathrm{Var}}[\widehat{\widehat{Y}}_j(z;\alpha \mid B) \mid Q_j=1] \mid Q_j=1\} = \mathrm{Var}[\widehat{\widehat{Y}}_j(z;\alpha \mid B) \mid Q_j=1].$$

where

$$\widehat{\mathrm{Var}}[\widehat{\widehat{Y}}_j(1;\alpha \mid B) \mid Q_j=1] \equiv \left(1-P_\alpha^j\right)\frac{\mathbb{I}_{[d_j\in B]}\sum_{i=1}^{n_j}\left[Y_{ij}-\widehat{\widehat{Y}}_j(1;\alpha \mid B)\right]^2 Z_{ij}}{(n_jP_\alpha^j-1)n_jP_\alpha^j}$$

with $\widehat{\mathrm{Var}}[\widehat{\widehat{Y}}_j(0;\alpha \mid B) \mid Q_j=1]$ and $\widehat{\mathrm{Var}}[\widehat{\widehat{Y}}_j(z;\gamma \mid B) \mid Q_j=0]$ defined similarly.

**Proof Theorem 1 in this setting**

Under assumptions a-d, Theorem 1 in this setting follows directly from Hudgens and Halloran [2008] Theorem 4, as if $d_j \in B$, then $\mathrm{E}\{\widehat{\mathrm{Var}}[\widehat{\widehat{Y}}_j(z;\alpha \mid B) \mid Q_j=1] \mid Q_j=1\} = \mathrm{Var}[\widehat{\widehat{Y}}_j(z;\alpha) \mid Q_j=1]$ by Theorem 4 of Hudgens and Halloran [2008] and otherwise it has zero variance because its value is always zero.

Similarly, under assumptions a-d, if $d_j$ is not in $B$, then $\mathrm{E}\{\widehat{\mathrm{Var}}[\widehat{\widehat{Y}}_j(z;\alpha \mid B) \mid Q_j=1] \mid Q_j=1\} = 0$ because its value is always zero. if $d_j \in B$, then, $\mathrm{E}\{\widehat{\mathrm{Var}}[\widehat{\widehat{Y}}_j(z;\alpha \mid B) \mid Q_j=1] \mid Q_j=1\} = \mathrm{E}\{\widehat{\mathrm{Var}}[\widehat{\widehat{Y}}_j(z;\alpha) \mid Q_j=1] \mid Q_j=1\} = \mathrm{Var}[\widehat{\widehat{Y}}_j(z;\alpha \mid B) \mid Q_j=1]$.

**Theorem 2** $\mid B$

Assuming that all $w_{ij} \in b$, thus we are only conditioning on $d_j \in B$, then under assumptions a-d and $M_B > 0$ and $nPr_\alpha - 1 > 0$

$$\mathrm{E}\{\widehat{\mathrm{Var}}[\widehat{\overline{Y}}(z;\alpha \mid B)]\} = \mathrm{Var}[\widehat{\overline{Y}}(z;\alpha \mid B)].$$

where

$$\widehat{\mathrm{Var}}[\widehat{\overline{Y}}(z;\alpha \mid B)] \equiv (1 - Pr_\alpha) \frac{\sum_{j=1}^{J} \mathbb{I}_{[Q_j=1]} \left[\widehat{\overline{Y}}_j(z;\alpha \mid B)(J/M_B) - \widehat{\overline{Y}}(z;\alpha \mid B)\right]^2}{(JPr_\alpha - 1)JPr_\alpha} + \frac{1}{Pr_\alpha M_B^2} \sum_{j=1}^{J} \widehat{\mathrm{Var}}[\widehat{Y}_j(z;\alpha \mid B)] \mathbb{I}_{[Q_j=1]}$$

with $\widehat{\mathrm{Var}}[\widehat{\overline{Y}}(z;\gamma \mid B)]$ defined similarly.

Follows in the same manner as Theorem 2 above, given Theorem 1 under $\mid B$.

**Theorem 1** $\mid B, b$

Under assumptions a-d and $M_{j,b} > 0$ and $n_j P_\alpha - 1 > 0$

$$\mathrm{E}\{\widehat{\mathrm{Var}}[\widehat{\overline{Y}}_j(z;\alpha \mid B, b) \mid Q_j = 1] \mid Q_j = 1\} = \mathrm{Var}[\widehat{\overline{Y}}_j(z;\alpha \mid b) \mid Q_j = 1].$$

where

$$\widehat{\mathrm{Var}}[\widehat{\overline{Y}}_j(1;\alpha \mid B, b) \mid Q_j = 1] \equiv \mathbb{I}_{[d_j \in B]} \left(1 - P_\alpha^j\right) \frac{\sum_{i=1}^{n_j} Z_{ij} \left[Y_{ij} Z_{ij} \mathbb{I}_{[w_{ij} \in b]}(n_j/M_{j,b}) - \widehat{\overline{Y}}_j(1;\alpha \mid b)\right]^2}{(n_j P_\alpha^j - 1) n_j P_\alpha^j}$$

with $\widehat{\mathrm{Var}}[\widehat{\overline{Y}}_j(0;\alpha \mid B, b) \mid Q_j = 1]$ and $\widehat{\mathrm{Var}}[\widehat{\overline{Y}}_j(z;\gamma \mid B, b) \mid Q_j = 0]$ defined similarly.

Follows from above.

**Theorem 2** $\mid B, b$

Under assumptions a-d and $M_{B,b} > 0$ $nPr_\alpha - 1 > 0$ and $n_j P_\alpha - 1 > 0$ for all $j$

$$\mathrm{E}\{\widehat{\mathrm{Var}}[\widehat{\overline{Y}}(z;\alpha \mid B, b)]\} = \mathrm{Var}[\widehat{\overline{Y}}(z;\alpha \mid B, b)].$$

where

$$\widehat{\text{Var}}[\widehat{\overline{Y}}(z;\alpha \mid B,b)] \equiv (1-Pr_\alpha)\,\frac{\sum_{j=1}^{J}\mathbb{I}_{[Q_j=1]}\left[\widehat{\overline{Y}}_j(z;\alpha \mid B,b)(J/M_{B,b})-\widehat{\overline{Y}}(z;\alpha \mid B,b)\right]^2}{(JPr_\alpha-1)JPr_\alpha}$$

$$+\frac{1}{Pr_\alpha M_{B,b}^2}\sum_{j\in\mathbb{J}^b}\widehat{\text{Var}}[\widehat{Y}_j(z;\alpha \mid B,b)]\mathbb{I}_{[Q_j=1]}$$

with $\widehat{\text{Var}}[\widehat{\overline{Y}}(z;\gamma \mid B,b)]$ defined similarly.

Follows from above.

# References

Michael G Hudgens and M Elizabeth Halloran. Toward causal inference with interference. *Journal of the American Statistical Association*, 103(482):832–842, 2008.
